# Supplementary material for: A data-based comparison of methods for reducing the peak volume flow rate in a district heating system
Source: arXiv:2403.16738 source file (2024-03-25)
Supplement: Supplementary file 1 [file appendix-graphs.tex]

Here's some equations we discussed during the project:

\subsection{Additional heat supply capacity}
\begin{equation}
    \dot{Q}_\text{additional} = \Delta \dot{V} \cdot \rho \cdot c_p \cdot \left( T_\text{SL,DH,max}- 50 ^\circ C \right)
\end{equation}

\begin{equation}
    \Delta \dot{V} = \left( \dot{V}_\text{max,original} - \dot{V}_\text{max,altered} \right)
\end{equation}

\begin{equation}
    \dot{Q}_\text{rel,additional} = \dot{Q}_\text{additional} / \dot{Q}_\text{max,original}
\end{equation}

\subsection{Pumping power estimation}
\begin{equation}
    {P}_\text{el,pu} = \frac{\frac{\dot{V_\text{CHP}}}{3600} \cdot dP \cdot 100} {\eta_\text{pump}} \cdot \frac{\dot{V_\text{subgrid}}}{\dot{V_\text{CHP}}}
    \label{eq:pumping power}
\end{equation}
\begin{equation}
    dP = 0.00001 * \dot{V_\text{CHP}}^{1.84}
\end{equation}
where ${P}_\text{el,pu}$ is the electric power of the pump in $kW$, $\dot{V}$ is flow in $\frac{m^3}{h}$, $dP$ is differential pressure in $bar$ or $\frac{kg \cdot 10^5}{m \cdot s^2}$ (can be retrieved from measurement data at the CHP plant) and $\eta_\text{pump}$ is the pump efficiency (could be assumed to be constant, i.e. 0.7)

\textcolor{blue}{Assuming that \eqref{eq:pumping power} has $dP$ proportional to $\dot{V}^2$, we can calculate an estimate of the improvement by calculating}
\begin{equation}
    \eta_\text{improvement} = 1 - \frac{\sum_{t=1}^{8760} \dot{V}_\text{new}(t)^3 }{ \sum_{t=1}^{8760} \dot{V}_\text{old}(t)^3}
\end{equation}
